# Supplementary material for: vMF-Contact: Uncertainty-aware Evidential Learning for Probabilistic Contact-grasp in Noisy Clutter
Source: arXiv:2411.03591 source file (2025-03-16)
Supplement: Supplementary file 1 [file supplementary.tex]

\section{Supplementary provements}

The von Mises-Fisher (vMF) distribution is one of the exponential family distributions on the \((p-1)\)-dimensional unit sphere in \(\mathbb{R}^p\). 
In the area of robotic manipulation, Liu et al.~\cite{liu2024efficient} utilized the Power Spherical (PS) distribution~\cite{de2020power} to model the baseline vectors of contact grasp representation~\cite{sundermeyer2021contact} as a substitute for the vMF distribution, owing to its stability and faster sampling speed compared to Gibbs sampling. Here we consider modeling the 3-D (\(p=3\)) vMF distribution, which is systematically analyzed in~\cite{straub2017bayesian}:
\begin{align*}
\mathrm{vMF}(x; \mu, \kappa) =  Z(\kappa) \exp(\kappa \mu^\top x),  Z(\kappa) = \frac{\kappa}{4\pi \sinh(\kappa)}.
\end{align*}

Given random mean parameter \(\mu\) and constant \(\kappa\), the conjugate prior of vMF distribution is another vMF distribution as \(\mathrm{vMF}(\mu | \mu_0, \kappa_0)\)~\cite{nunez2005bayesian}. When directional data \(\mathbf{x} = \{x_i\}_{i=1}^N\) is collected, the posterior distribution can be derived by:
\begin{align*}
p(\mu \mid \mathbf{x}; \kappa, \mu_0, \kappa_0) \propto \mathrm{vMF}(\mu | \mu_0, \kappa_0) \prod_{i=1}^N \mathrm{vMF}(x_i| \mu, \kappa).
\end{align*}

In addition, in cases where numerical Monte Carlo (MC) sampling: \(\mathbb{E}_{{\theta} \sim \mathbb{Q}_{\text{post.}}}[f(\theta^{s})] \approx \frac{1}{S} \sum_{s=1}^{S} f(\theta^{s}) \) is unavoidable due to analytical intractability, PS distributions can be ideal surrogates with the same parameterizations as the vMF posterior \(\mathbb{Q}_{\text{post.}}=\text{vMF} (\mu \mid \mathbf{x}; \kappa, \mu_0, \kappa_0)\). However, it is important to note that the conjugate prior of the PS distribution can only be derived in close form~\cite{de2020power}, which may impose limitations on analytical stability.

For joint conjugate prior between \(\mu\) and \(\kappa\) one can only derive \(p(\mu, \kappa \mid \mathbf{x}; \mu_0, a, b)\) with \(0<a<b\) up to proportionality. While there's no analytical solution for normalization of the posterior density as well as statistics in terms of e.g. marginalization, entropy, maximum likelihood, etc~\cite{nunez2005bayesian}. For this reason, we only consider vMF with a fixed concentration parameter \(\kappa\) in the following derivations.

\subsection{Evidential learning with natural posterior networks (NatPN)}

We follow the same regime to formulate the evidential learning with natural posterior update as Charpentier et al.~\cite{charpentier2021natural}. Since vMF belongs to exponential family distribution the corresponding natural parameters can be interesting. Consider the following formulation as the general expression of the exponential family~\cite{bishop2006pattern}:
\begin{align*}
    f(x; \mathbf{\theta}) = h(x) \exp\left( \eta(\mathbf{\theta})^\top T(x) - A(\mathbf{\theta}) \right).
\end{align*}

We can rewrite 3D vMF density as:
\begin{align*}
    f(x; \kappa \mathbf{\mu}) = \exp(\kappa \mathbf{\mu}^\top x + \log Z(\kappa)),
\end{align*}
with natural parameter: \(\eta(\kappa \mathbf{\mu}) = \kappa \mathbf{\mu}\), sufficient statistic: \(T(x) = x\), log-partition function: \(A(\kappa \mathbf{\mu}) = -\log Z(\kappa)\). The posterior distribution:
\begin{align*}Q(\theta | \chi^{(\cdot)}, m^{(\cdot)}) = \eta(\chi^{(\cdot)}, n) \exp \left( m^{(\cdot)} \theta^\top \chi^{(\cdot)} - m^{(\cdot)} A(\theta) \right),
\end{align*}
with the corresponding update:
\begin{align*}
    \mathbf{\chi}^{\text{post}, (i)} = \frac{m^{\text{prior}} \mathbf{\chi}^{\text{prior}} + m^{(i)} \mathbf{\chi}^{(i)}}{m^{\text{prior}} + m^{(i)}}, \ m^{\text{post}, (i)} = m^{\text{prior}} + m^{(i)}
\end{align*}
exits for vMF as a member of the exponential family. With \(\chi^{\text{prior}} = \mu_0\), \(m^{\text{prior}} = \kappa_0\) and \( \eta(\chi^{(\cdot)}, m)\) as normalization factor, we may perform the following posterior update for vMF as well:
\begin{align*}
    \mathbf{\mu}^{\text{post}}_i = \frac{\kappa_0 \mathbf{\mu}_0 + m_i x_i}{\kappa_0 + m_i}, \ \kappa^{\text{post}}_i = \kappa_0 + m_i, \  m_i \equiv N_H p(x_i).
\end{align*}

Here \(m_i\) represents the evidence (or pseudo-count) given \(N_H\) as the scaling factor (or certainty budget). The evidence inherently contains epistemic uncertainty. Intuitively, the posterior update can be considered as the linear interpolation between the prior and observed data.

\subsubsection{Maximum a-posterior}

One important statistic is the maximum a-posterior (MAP). Here the posterior distribution for \(\mu\) and \(\kappa\) given the priors \( \mu_0 \) and \( \kappa_0 \) can be written as:
\begin{align*}
p(\mu, \kappa \mid \mathbf{x}; \mu_0, \kappa_0) \propto p(\mathbf{x} \mid \mu, \kappa) p(\mu \mid \mu_0, \kappa_0).
\end{align*}

Given the vMF likelihood \(p(\mathbf{x} ; \mu, \kappa) = Z(\kappa) \exp(\kappa \mathbf{x}^\top \mu) \) and prior \( p(\mu ; \mu_0, \kappa_0) = Z(\kappa_0) \exp(\kappa_0 \mu_0^\top \mu) \)
\begin{align*}
    \log p(\mu \mid \mathbf{x}; \kappa, \mu_0, \kappa_0) \propto \kappa \mathbf{x}^\top \mu + \kappa_0 \mu_0^\top \mu, 
\end{align*}
with \(\log Z(\kappa_0), \log Z(\kappa)\) as constants. Since \(\mu\) is a unit vector, the maximum occurs when:
\begin{align*}
\vartheta_N = \kappa_0 \mu_0 + \kappa \mathbf{x}, \
\mu_{\text{MAP}} = \frac{\vartheta_N}{\| \vartheta_N \|_2}.
\end{align*}

This aligns with the posterior mean from~\cite{straub2017bayesian} , where \(p(\mu \mid \mathbf{x}; \kappa, \mu_0, \kappa_0) = \mathrm{vMF} \left( \mu; \frac{\vartheta_N}{\| \vartheta_N \|_2}, \| \vartheta_N \|_2 \right)
\). 

\subsubsection{Bayesian loss}
\label{ell_prove}
In evidential deep learning, one needs to optimize the following objective as "Bayesian loss":
\begin{equation}
\label{BL}
\mathcal{L}^{post}_i = -  \underbrace{\mathbb{E}_{\boldsymbol{\theta} \sim \mathbb{Q}_{\text{post.}}} \left[ \log \mathbb{P}(x_i \mid \boldsymbol{\theta}) \right]}_{\text{(i)}} - \underbrace{\mathbb{H}[\mathbb{Q}_{\text{post.}}]}_{\text{(ii)}},
\end{equation}
where (i) is the expected log-likelihood and (ii) denotes the entropy of the predicted posterior distribution \(\mathbb{Q}_{\text{post.}}\). In terms of vMF posterior, the entropy can be derived by~\cite{charpentier2021natural}:
\begin{align}\label{entropy}
    \mathbb{H} (\mathrm{vMF}(\cdot ; \mu_0, \kappa_0))= -\log  Z(\kappa_0) - \frac{\kappa_0}{\tanh (\kappa_0)} + 1.
\end{align}

This represents the epistemic uncertainty, which is independent of the mean direction \(\mu\).

As for the expected log-likelihood of vMF distribution, we would like to derive the analytical formulation of expected log-likelihood \(\kappa\):
\label{ELL}
\begin{align*}
& \mathbb{E}_{\mu \sim \mathbb{Q}(\mu_0, \kappa_0)} \left[ \log \mathbb{P}(x_i \mid \mu) \right] \\  =  &  \int_{\mu \in S^2} \mathrm{vMF}(\mu; \mu_0, \kappa_0) \log \mathrm{vMF}(x_i; \mu, \kappa) \, d\mu \\
=  & \int_{\mu \in S^2} Z(\kappa_0) \exp(\kappa_0 \mu_0^\top \mu) \left( \log Z(\kappa) + \kappa x_i^\top \mu \right) d\mu \\
=  & Z(\kappa_0) [ \log Z(\kappa)\underbrace {\int_{\mu \in S^2} \exp(\kappa_0 \mu_0^\top \mu)  \, d\mu}_{\textcircled{1}} \\ &+  \kappa \underbrace {\int_{\mu \in S^2} \exp(\kappa_0 \mu_0^\top \mu) x_i^\top \mu \, d\mu}_{\textcircled{2}} ].
\end{align*}

Due to rotational symmetry, we can assume \(\mu_0 = (0,0,1)^\top\). Transform vector \(\mu\) to cartesian coordinates using \(
\mu = (\sin \theta \cos \phi, \sin \theta \sin \phi, \cos \theta)^\top
\), the term \(\textcircled{1}\) gives:
\begin{align*}
&  \int_{0}^{2\pi} \int_{0}^{\pi} \exp(\kappa_0 \cos \theta) \sin \theta \, d\theta \, d\phi 
\\=& 2\pi  \int_{0}^{\pi} \exp(\kappa_0 \cos \theta) \sin \theta \, d\theta = 4\pi   \frac{\sinh(\kappa_0)}{\kappa_0}.
\end{align*}

For generality, we need to apply the same transformation to the data \( x_i \) as we would transform any \(\mu_0 \in S^2\) to align with the z-axis. This is not necessary for \(\mu\) due to the integral over the whole sphere.
Suppose \(
x^{\text{proj}}_{i} = (x_{ia}, x_{ib}, x_{ic})^\top
\),  the term \(\textcircled{2}\) with \(x^{\text{proj}}_{i}\) as the data after transformation: 
\begin{align*}
& \int_{0}^{2\pi} \int_{0}^{\pi} \exp(\kappa_0 \cos \theta) x^\top \left( \begin{matrix} \sin \theta \cos \phi \\ \sin \theta \sin \phi \\ \cos \theta \end{matrix} \right) \sin \theta \, d\theta \, d\phi \\
=&  \int_{0}^{2\pi} \int_{0}^{\pi} \exp(\kappa_0 \cos \theta) \biggl( \underbrace{\sin \theta \cos \phi  x_{ia}  + \sin \theta \sin \phi  x_{ib}}_{\text{integral as } 0 \text{ over } \phi} \biggr. \\
 & \quad + \biggl.\text{}\cos \theta  x_{ic} \biggr) \sin \theta \, d\theta \, d\phi \\
=& 2\pi  x_{ic} \int_{0}^{\pi} \exp(\kappa_0 \cos \theta) \cos \theta \sin \theta  \,  d\theta \\
=& 4\pi  x_{ic} \left( \frac{\cosh(\kappa_0)}{\kappa_0} - \frac{\sinh(\kappa_0)}{\kappa_0^2} \right)
\end{align*}

We can see that terms \(x_{ia}\) and \(x_{ib}\) are removed since the integral over \(\sin(\phi)\) and \(\cos(\phi)\) cancel out the positive and negative halves in range \(0-2\pi\). Finally, combine \(\textcircled{1}\) and \(\textcircled{2}\) together:
\begin{align*}
& \mathbb{E}_{\boldsymbol{\theta} \sim \mathbb{Q}_{\text{post.}}} \left[ \log \mathbb{P}(x_i \mid \boldsymbol{\theta}) \right] \\
=& Z(\kappa_0) \left[ 4\pi \log Z(\kappa)  \frac{\sinh(\kappa_0)}{\kappa_0} + 4\pi \kappa x_{ic} \left( \frac{\cosh(\kappa_0)}{\kappa_0} - \frac{\sinh(\kappa_0)}{\kappa_0^2} \right) \right]\\
=& \frac{4\pi Z(\kappa_0)}{\kappa_0} \left[ \log Z(\kappa) \sinh(\kappa_0) + \kappa x_{ic} \cosh(\kappa_0) - \kappa x_{ic} \frac{\sinh(\kappa_0)}{\kappa_0} \right] \\
=& \log Z(\kappa) - \frac{\kappa x_{ic}}{\kappa_0} + \frac{\kappa x_{ic}}{\tanh( \kappa_0)}
\end{align*}
and \(x_{ic}\) is the projection of \(x_{i}\) on any \(\mu_0 \in S^2\) as \(x_{ic} =\frac{ x_{i}^\top\mu_0}{\|\mu_0\|}  \) with \(\|\mu_0\| = 1 \). This finally gives:
\begin{align*}
\label{ell}
&\mathbb{E}_{\mu \sim \mathbb{Q}(\mu_0, \kappa_0)} \left[ \log \mathbb{P}(x_i \mid \mu) \right] \\ =& \log Z(\kappa) + \left( \frac{1}{\tanh( \kappa_0)} - \frac{1}{\kappa_0} \right) \kappa  x_{i}^\top\mu_0
\end{align*}

\subsection{Short analysis of Bayesian loss}
As in the aforementioned Bayesian loss (Eq.\ref{BL}), if we first put our attention on the expected log-likelihood (as just derived in Eq.\ref{ell}), where, intuitively, the normalizer \(\log Z(\kappa)\) achieves maximum when  \(\kappa = 0\), imposing high \textcolor{blue}{aleatoric uncertainty} for small \(\kappa_0\). But when \(\kappa_0 >> 0\),  \( \frac{1}{\tanh( \kappa_0)} - \frac{1}{\kappa_0} \approx 1 \) (which also means low epistemic uncertainty due to the posterior update \(\kappa_0 \leftarrow \kappa_0 + m^i\)), to maximize the expected log-likelihood, there exists a balance between this normalizer \(\log Z(\kappa)\) and \(\kappa x_{i}^\top\mu_0\), where \(\kappa\) is weighted by the alignment between data \(x_i\) with the prior/posterior mean direction \(\mu_0\). While in case the posterior has a small concentration \(\kappa_0\) (or high epistemic uncertainty), the second term will also be down-weighted. 

In terms of learning \(\kappa_0\) (or \(n_i\) in specific), the expected log-likelihood intends to reduce the epistemic uncertainty by maximizing \( \frac{1}{\tanh( \kappa_0)} - \frac{1}{\kappa_0}\), while in Bayesian loss, this is balanced through the maximization of the entropy \(\mathbb{H} (\mathrm{vMF}(\cdot; \mu_0, \kappa_0))\) in Eq.\ref{entropy}.
